# Supplementary material for: Parendi: Thousand-Way Parallel RTL Simulation
Source: arXiv:2403.04714 source file (2025-03-16)
Supplement: Supplementary file 1 [file appendix.tex]

\section{Appendix}

\subsection{Performance Comparison}

\tabRef{perf_smackdown} contains detailed performance numbers for each of the designs we considered in~\secRef{evaluation}.

\subsection{Compilation time and Memory Usage}

\SimName and Verilator have vastly different compile time and memory usage profiles.

Let us first consider memory usage (memory used to compile a design).
\figRef{memory_usage_x64} and \figRef{memory_usage_ipu} shows how Verilator's and \SimName's memory usages varies for different design size and available parallelism.
\SimName shows a slow increase in memory usage, whereas Verilator blows up and uses more than one TiB.

\figRef{compile_time_ipu} and~\figRef{compile_time_x64} show how the compile time varies for different designs and available parallelism.
While Verilator is really fast for small designs with few number of threads, it becomes incredibly slow for larger ones with more threads.
In contrast, \SimName shows a relatively flat profile. Compile time increases only slightly, despite compiling code to up to 5888 tiles.

\subsection{Cost Analysis}
To analyze the cost of running simulation using \SimName or Verilator we consider running simulation in the public cloud using IPUs or x64, respectively.
For Verilator we take a 32-core Dav4 instance from Microsoft Azure (AMD EPYC 7452) and an IPU-POD4 classic from GCore (M2000).
These machines cost \$1.536 and \$2.13 per hour, respectively.

We consider running each benchmark for 1 billion cycles (e.g., 1 second of simulation assuming a 1~GHz clock).
\figRef{cost_compare} shows how much each simulation will cost on the respective hardware.
For larger designs, the IPU is more cost-effective since a 4 IPUs cost only $39\%$ more than a 32-core virtual machine, but they are 3--4$\times$ faster.
Consequently, simulation finishes earlier and the total cost reduces.

\begin{figure}[h]
    \centering
    \includegraphics[width=\columnwidth]{figures/gen/memory_usage_x64.pdf}
    \caption{Verilator's memory usage.}
    \label{fig:memory_usage_x64}
\end{figure}
\begin{figure}[h]
    \centering
    \includegraphics[width=\columnwidth]{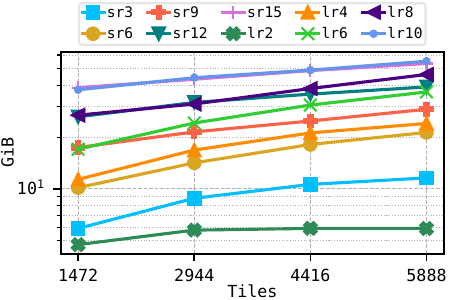}
    \caption{\SimName's memory usage.}
    \label{fig:memory_usage_ipu}
\end{figure}
\begin{figure}[h]
    \centering
    \includegraphics[width=\columnwidth]{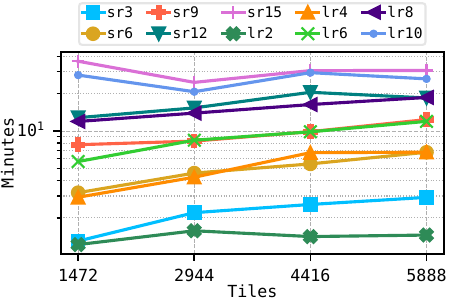}
    \caption{\SimName's compile time.}
    \label{fig:compile_time_ipu}
\end{figure}

\begin{figure}[h]
    \centering
    \includegraphics[width=\columnwidth]{figures/gen/compile_time_x64.pdf}
    \caption{Verilator's compile time.}
    \label{fig:compile_time_x64}
\end{figure}
\begin{figure}[h]
    \centering
    \includegraphics[width=\columnwidth]{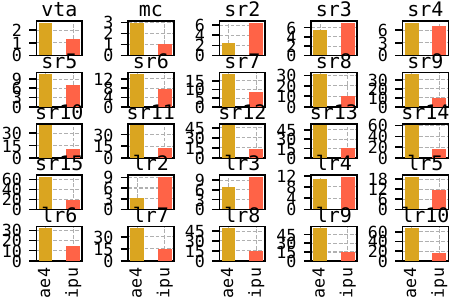}
    \caption{Cost of simulating 1 billion cycles in \$. \sk{Y-axis needs a legend, even if in the caption.}}
    \label{fig:cost_compare}
\end{figure}

\subsection{Partitioning Strategies}
So far, we have used the partitioning strategy outlined in~\secRef{partitioning}.
This section considers alternative strategies for partitioning \fibers within and across IPUs.

\subsubsection{Single-IPU}
We presented a bottom-up strategy in~\secRef{partitioning} that conservatively merges tiny \fibers to make \threads.
Recent work proposes casting this problem as a hypergraph partitioning problem where hypergraph nodes represent clusters of computation and hyperedges represent duplicated clusters across \fibers~\cite{repcut}.
The goal of this proxy problem is to find a balanced partitioning of clusters while minimizing duplication.
We implemented this strategy in \SimName as an alternative for users.
\figRef{merge_compare_breakdown} compares our default bottom-up (\textbf{B}) strategy with hypergraph partitioning (\textbf{H}) on a single IPU (1472-way partitioning).
The vertical axis shows the normalized number of IPU machine cycles per RTL cycle (i.e., reciprocal of rate; lower is better).
Interestingly, neither strategy is objectively better.
Bottom-up performs best with \smallrocket{N}, whereas hypergraph partitioning performs better with \largerocket{N} in some cases.

\begin{figure}[h]
    \centering
    \includegraphics[width=\columnwidth]{./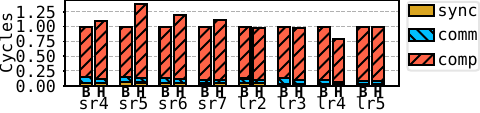}
    \caption{Comparison of our method with the hypergraph partitioning from repcut~\cite{repcut}.
        We compare our bottom-up (\textbf{B}) \fiber merge strategy with the hypergraph (\textbf{H}) used in repcut.
        The vertical axis shows IPU machine cycles per RTL cycle, normalized to \textbf{B} (lower is better).}
    \label{fig:merge_compare_breakdown}
\end{figure}

\subsubsection{Multi-IPU partitioning}

\figRef{device_partitioning_compare} compares three strategies for multi-device partitioning over 4 IPUs:
\begin{itemize}
    \item Pre: partition \fibers across IPU before they are merged into \threads (default \SimName strategy)
    \item Post: partition \threads across IPU, i.e., after \fibers are merged into \threads
    \item None: do not partition \fibers or \thread, i.e., multi-IPU oblivious
\end{itemize}

Not partitioning \fibers or \threads across IPUs yields objectively inferior performance as expected.
However, partitioning \fibers works better than partitioning \threads, too.
This is because, during the merge, we may suboptimally absorb some \emph{good cuts} and land in a region of the design space that is only locally optimal.
Conversely, partitioning \fibers before the merge helps us better optimize globally.

\begin{figure}[h]
    \centering
    \includegraphics[width=\columnwidth]{./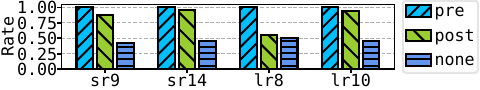}
    \caption{Normalized simulation rate for 4-IPU partitioning strategies.
        Partitioning \fibers \textbf{pre} merge performs better than partitioning \threads \textbf{post} merge.
        Being oblivious to the muli-IPU setup (\textbf{none}), yields vastly inferior results.
        \me{TODO: Add another plot that show the cut size in each.}
    }
    \label{fig:device_partitioning_compare}
\end{figure}

\clearpage
% \input{sections/table_smackdown.tex}
% \begin{figure}
%     \subfloat[\SimName] {
%         \label{fig:memory_usage_ipu}
%         \includegraphics[width=\columnwidth]{figures/gen/memory_usage_ipu.pdf}
%     }\\
%     \subfloat[Verilator] {
%         \label{fig:memory_usage_x64}
%         \includegraphics[width=\columnwidth]{figures/gen/memory_usage_x64.pdf}
%     }
%     \caption{\SimName's and Verilator's memory usage for a few designs.}
%     \label{fig:memory_usage}
% \end{figure}

% \begin{figure}
%     \subfloat[\SimName] {
%         \label{fig:compile_time_ipu}
%         \includegraphics[width=\columnwidth]{figures/gen/compile_time_ipu.pdf}
%     }\\
%     \subfloat[Verilator] {
%         \label{fig:compile_time_x64}
%         \includegraphics[width=\columnwidth]{figures/gen/compile_time_x64.pdf}
%     }
%     \caption{\SimName's and Verilator's compile time.}
%     \label{fig:compile_time}
% \end{figure}
